# Supplementary material for: Understanding the Acceleration Phenomenon via High-Resolution Differential Equations
Source: arXiv:1810.08907 source file (2018-11-01)
Supplement: Supplementary file 1 [file proof73.tex]

%\begin{proof}[Proof of Theorem~\ref{thm: ODE_generalize_>3}]
\subsection{Proof of Theorem~\ref{thm: ODE_generalize_>3}}
\label{subsec: proof_gamma_3_ODE}

With the inequality for any function $f(x) \in \mathcal{F}_{L}^{2}(\mathbb{R}^{n})$,
$$
f(x^{\star}) \geq f(X(t)) + \left\langle \nabla f(X(t)), x^{\star} - X(t) \right\rangle + \frac{1}{2L} \left\| \nabla f(X(t)) \right\|^{2},
$$
the time derivative of the Lyapunov function~(\ref{eqn: energy_functional_ode_>3}) along the trajectory of the equation~(\ref{eqn: generalize_NAGM-C_SES}) can be estimated as below
$$
\begin{aligned}
\frac{\dd \mathcal{E}(t)}{\dd t} & =       \left( 2t - \sqrt{S} \right) \left( f(X(t)) - f(x^{\star}) \right)+ t \left( t - \sqrt{S} \right) \left\langle \nabla f(X(t)), \dot{X}(t) \right\rangle \\
                                         & \quad + \left\langle \left( \sqrt{S} - t\right) \nabla f(X(t))   , (\gamma - 1) (X(t) - x^{\star}) + t \left( \dot{X}(t) + \sqrt{S} \nabla f(X(t)) \right)  \right\rangle \\
                                         & \leq  (\gamma - 1) (\sqrt{S} - t) \left\langle \nabla f(X(t)), X(t) - x^{\star} \right\rangle  + (2t - \sqrt{S}) \left( f(X(t)) - f(x^{\star}) \right) \\
                                         &\quad + \sqrt{S} t \left( \sqrt{S} - t \right) \left\| \nabla f(X(t)) \right\|_{2}^{2} \\
                                         & \leq   - \left[ (\gamma - 3)t - \sqrt{S} (\gamma - 2)  \right]\left( f(X(t)) - f(x^{\star}) \right) + \sqrt{S} t \left( \sqrt{S} - t \right) \left\| \nabla f(X(t)) \right\|^{2}
\end{aligned}
$$
Since $\left\| \nabla f(X(t)) \right\|^{2} \geq 0$ and $f(X(t)) - f(x^{\star}) \geq 0$, then when $t \geq t_{0} = \sqrt{S}(\gamma - 2)/ (\gamma - 3)$, we have
$$
\left\{ \begin{aligned}
          & f(X(t)) - f(x^{\star}) \leq  \frac{\mathcal{E}(t_{0})}{t (t - \sqrt{S})} \\
          & \int_{t_{0}} ^{t} \left[ (\gamma - 3)u - \sqrt{S} (\gamma - 2)  \right]\left( f(X(u)) - f(x^{\star}) \right) + \sqrt{S} u \left( u - \sqrt{S}  \right) \left\| \nabla f(X(u)) \right\|^{2} du \leq \mathcal{E}(t_{0})
         \end{aligned} \right.
$$
With some basic calculations, we complete the proof.
%\end{proof}
