# Supplementary material for: Understanding the Acceleration Phenomenon via High-Resolution Differential Equations
Source: arXiv:1810.08907 source file (2018-11-01)
Supplement: Supplementary file 2 [file wproof71_delete.tex]

\bin{ \textbf{This part has been cut.}
\begin{proof}[Theorem~\ref{thm: ODE_generalize_=3}]
Consider the Lyapunov function defined as
\begin{equation}
\label{eqn: lypunov_NAGM-C_first-order_ode_=3}
\mathcal{E}(t) = t(t - \gamma_{2}) \left( f(X(t)) - f(x^{\star}) \right) + \frac{1}{2} \left\| 2 (X(t) - x^{\star}) + t ( \dot{X}(t) + \gamma_{2} \nabla f(X(t)) ) \right\|^{2}.
\end{equation}
With the inequality for convex function $f(x) \in \mathcal{F}_{L}^{1,1}$, 
$$
f(x^{\star}) \geq f(X(t)) + \left\langle \nabla f(X(t)), x^{\star} - X(t) \right\rangle + \frac{1}{2L} \left\| \nabla f(X(t)) \right\|^{2}
$$
the time derivative of the Lyapunov function~(\ref{eqn: lypunov_NAGM-C_first-order_ode_=3}) is 
$$
\begin{aligned}
\frac{d \mathcal{E}(t)}{dt} & = \left(2t - \gamma_{2}\right) \left( f(X(t)) - f(x^{\star}) \right) + t(t - \gamma_{2}) \left\langle \nabla f(X(t)), \dot{X}(t) \right\rangle \\
                                         &\quad + \left\langle 2 (X(t) - x^{\star}) + t ( \dot{X}(t) + \gamma_{2} \nabla f(X(t)) ), (\gamma_{2} - t) \nabla f(X(t)) \right\rangle    \\
                                         & = \left(2t - \gamma_{2}\right) \left( f(X(t)) - f(x^{\star}) \right) + 2(\gamma_{2} - t) \left\langle X(t) - x^{\star}, \nabla f(X(t)) \right\rangle \\
                                         & \quad - \gamma_{2}t(t - \gamma_{2})\left\| \nabla f(X(t)) \right\|^{2} \\
                                         & \leq \gamma_{2} \left( f(X(t)) - f(x^{\star}) \right) - \left(\gamma_{2}t + \frac{1}{L}\right)(t - \gamma_{2})\left\| \nabla f(X(t)) \right\|^{2} \\
                                         & \leq \frac{\gamma_{2}}{t(t - \gamma_{2})} \mathcal{E}(t) - \gamma_{2} t (t - \gamma_{2})\left\| \nabla f(X(t)) \right\|^{2}
\end{aligned}
$$
Furthermore, the simple calculation tells us that
$$
\begin{aligned}
\frac{d}{dt} \left( \frac{t}{t - \gamma_{2}} \mathcal{E}(t) \right) & = \frac{ (t - \gamma_{2}) \left( \mathcal{E}(t) + t \dot{\mathcal{E}}(t) \right) - t \mathcal{E}(t)}{(t - \gamma_{2})^{2}} \\
                                                                               & = - \frac{\gamma_{2}}{(t - \gamma_{2})^{2}} \mathcal{E}(t) + \frac{t}{t - \gamma_{2}} \dot{\mathcal{E}}(t) \\
                                                                               & \leq - \frac{\gamma_{2}}{(t - \gamma_{2})^{2}} \mathcal{E}(t) + \frac{t}{t - \gamma_{2}} \left[ \frac{\gamma_{2}}{t(t - \gamma_{2})} \mathcal{E}(t) -  \gamma_{2} t (t - \gamma_{2})\left\| \nabla f(X(t)) \right\|^{2} \right] \\
                                                                               & = - \gamma_{2} t^{2}\left\| \nabla f(X(t)) \right\|^{2}
\end{aligned}
$$
Since $\left\| \nabla f(X(t)) \right\|^{2} \geq 0$ and $\mathcal{E}(t) \geq 0$, then when $t \geq 2\gamma_{2}$, we have
$$
\left\{ \begin{aligned}
         & f(X(t)) - f(x^{\star}) \leq \frac{\mathcal{E}(t)}{t (t - \gamma_{2})} \leq 2\mathcal{E}(2\gamma_{2})  \cdot \frac{1}{t^{2}}\\
         & \int_{2\gamma_{2}}^{t}  \gamma_{2}s^{2} \left\| \nabla f(X(s)) \right\|_{2}^{2} ds \leq  2\mathcal{E}(2\gamma_{2}) 
         \end{aligned} \right. 
$$
Hence, with some basic calculations, the proof is complete.
\end{proof}
}
