# Supplementary material for: Understanding the Acceleration Phenomenon via High-Resolution Differential Equations
Source: arXiv:1810.08907 source file (2018-11-01)
Supplement: Supplementary file 3 [file miscellaneous.tex]

\wjs{Give details on $O(\frac{L^2}{k^4})$. Point to the reference which proposes this rate and explain why this rate makes sense.} \bin{I cannot finish this work, so many problems are hard to understand.}

\begin{itemize}
\item 
\item \textbf{Lower Bound for Half-Dimension.} In~\cite[Theorem 2.1.7]{nesterov2013introductory}, it shows that for any first-order method and $f(x) \in \mathcal{F}_{L}^{\infty, 1} (\mathbb{R}^{n})$, when $1 \leq k \leq (1/2)(n - 1)$, the lower bound for function value is
\[
f(x_{k}) - f(x^{\star}) \geq \frac{3L \left\| x_{0} - x^{\star} \right\|^{2}}{32 (k + 1)^{2}}.
\]
Since $k \leq (1/2)(n - 1)$ is finite, then the expression below exists
\[
\min_{1 \leq k \leq (1/2)(n - 1)} \left\| x_{k} - x^{\star} \right\|^{2}.
\]
With the basic convex inequality, 
\[
f(x_{k}) - f(x^{\star}) \leq \left\langle \nabla f(x_{k}), x_{k} - x^{\star} \right\rangle \leq \left\| \nabla f(x_{k}) \right\| \left\| x_{k} - x^{\star} \right\| 
\]
we have
\[
\left\| \nabla f(x_{k}) \right\| \geq \frac{3L \left\| x_{0} - x^{\star} \right\|^{2}}{32 (k + 1)^{2}\left\| x_{k} - x^{\star} \right\| }\geq  \frac{3L \left\| x_{0} - x^{\star} \right\|^{2}}{32 (k + 1)^{2} \min\limits_{1 \leq k \leq (1/2)(n - 1)}  \left\| x_{k} - x^{\star} \right\| }= \Omega\left(\frac{L}{k^{2}}\right).
\]
\bin{For finite step, we also can have, when $1 \leq k \leq (1/2)(n - 1)$
\[
\left\| x_{k} - x^{\star} \right\| \leq \frac{C}{k}
\]
}
\end{itemize}
