# Supplementary material for: Understanding the Acceleration Phenomenon via High-Resolution Differential Equations
Source: arXiv:1810.08907 source file (2018-11-01)
Supplement: Supplementary file 4 [file proof70.tex]

\subsection{Proof of Theorem~\ref{thm: critical_case_ode}}
\label{subsec: critical_ode}

\begin{align*}
\frac{\dd \mathcal{E}(t)}{\dd t} & = \left[2t +  \left(\frac{3}{2} - C\right)\sqrt{s} \right] \left( f(X(t)) - f(x^{\star}) \right) +  t\left[ t + \left(\frac{3}{2} - C\right)\sqrt{s} \right] \left\langle \nabla f(X(t)), \dot{X}(t) \right\rangle \\
                                         &\quad + \left\langle 2 (X(t) - x^{\star}) + t \left( \dot{X}(t) + C\sqrt{s} \nabla f(X(t)) \right), -\left[ t + \left(\frac{3}{2} - C\right)\sqrt{s}\right] \nabla f(X(t)) \right\rangle    \\
                                         & = \left[2t +  \left(\frac{3}{2} - C\right)\sqrt{s} \right]  \left( f(X(t)) - f(x^{\star}) \right) - \left[2t -  (2C - 3) \sqrt{s}\right] \left\langle X(t) - x^{\star}, \nabla f(X(t)) \right\rangle \\
                                         & \quad - C\sqrt{s}t \left[ t + \left(\frac{3}{2} - C\right)\sqrt{s}\right]  \left\| \nabla f(X(t)) \right\|^{2}. 
\end{align*}

\begin{itemize}
\item When $C \leq 3/2$, simple
\item When $C > 3/2$, integral technique and initial point will be moved forward.
         \[
         t_{0} = \max\left\{ \frac{3}{2}\sqrt{s}, \left(C- \frac{3}{2}\right) \sqrt{s}\right\}
         \] 
         \begin{itemize}
         \item $3/2 < C < 3$
         \item $C \geq 3$
                  \[
                  t_{0} > \left(C- \frac{3}{2}\right) \sqrt{s}
                  \]
         \end{itemize}
\end{itemize}
